# Supplementary material for: Verification of a Generative Separation Kernel
Source: arXiv:2001.10328 source file (2020-05-14)
Supplement: Supplementary file 1 [file appendix-checking-algos.tex]

\section{Algorithms for Checking Condition $R$} 
\label{app:checking-algos}

Algorithm~\ref{alg:page_table_generation_check} shows our
algorithm for checking condition $R1$.
Recall that the physical memory components have already been
checked to be non-overlapping.

\begin{algorithm}
\begin{scriptsize}
\begin{algorithmic}[1]
\ForAll{\textit{s} in subjects}
\ForAll{\textit{m} in VmemComponents(s)}
\State $\page.LA$ = $m.LA$; \ \ // logical address
\State $\page . size$ = $m . size$;
\State $\page . PA$ = $m . PA$; \ \ // physical address
\State $\page . rwe$ = $m . rwe$; \ \ // permissions
\While{$\page . LA < m . LA + m . size$}
\If{$\pt_s(\page . LA) \neq \page . PA$}
\State Output(\enquote{Address mismatch});
\EndIf
\If{$\rwe_s(\page.LA) \neq \page.rwe$}
\State Output(\enquote{Rd/Write/Exec mismatch.});
\EndIf
%% \If{(pt\_ex(s, $\page.LA) \neq \page . ex$)}
%% \State Outuput(\enquote{Exec mismatch found.});
%% \EndIf
\State $\page . LA = \page . LA + page\_size$;
\State $\page . PA = \page . PA + page\_size$;
\EndWhile
\EndFor
\EndFor
\end{algorithmic}
\end{scriptsize}
\caption{Injectivity of page tables}
\label{alg:page_table_generation_check}
\end{algorithm}

Here $\rwe_s(a)$ is a function to check read/write/exec
permissions of the address $a$ in the page table of subject $s$.

The algorithm below checks condition $R_2$.
It ensures that no invalid virtual address in a subject's address
space is mapped to a physical address by the page table for $s$.
The algorithm exploits the way the translation is done through the
paging structures. This is shown in
Fig.~\ref{fig:paging-structure-1} and Fig.~\ref{fig:paging-structure-2}.

\begin{algorithm}
\begin{scriptsize}
\begin{algorithmic}[1]
\State Find page table file size; (MAXSIZE) 
\State Create an Int array of size MAXSIZE/8
\ForAll{\textit{s} in subjects}
\ForAll{\textit{m} in memorySegments(s)}
\ForAll {4$\mathrm { KB }$ page $p$ in $\mathrm { m }$}
\State   setBit (PTBitArray, PML4\_offset/8)
\State   setBit (PTBitArray, PDPTE\_offset/8)
\State   setBit (PTBitArray, PDE\_offset/8)
\State   setBit (PTBitArray, PTE\_offset/8)
\EndFor
\EndFor
\For{\texttt{$( \mathrm { x } = 0 ; \mathrm { x}<$ PTSize$( \textit{s}) ;  \mathrm { x}+=8 )$}}
        \If{$(($PagetableEntry $( \textit{s} , \mathrm { x } )  ! = 0 ) \&\&$ \\
        \hskip4.5em (TestBit(PTBitArray, $\mathrm {x}/8 ) == 0 )$)}
        \State Print ("Invalid Page Table Entry $@ \mathrm { x } / 8 ^ { \prime \prime } )$
\EndIf
\EndFor
\State Clear PTBitArray
\EndFor
\end{algorithmic}
\end{scriptsize}
\caption{Memory Gap Check}
\label{alg:memory_gap_check}
\end{algorithm}

Following diagrams explain paging in 64-bit mode.

\begin{figure}
\includegraphics[angle=90, origin=c,
  scale=0.6]{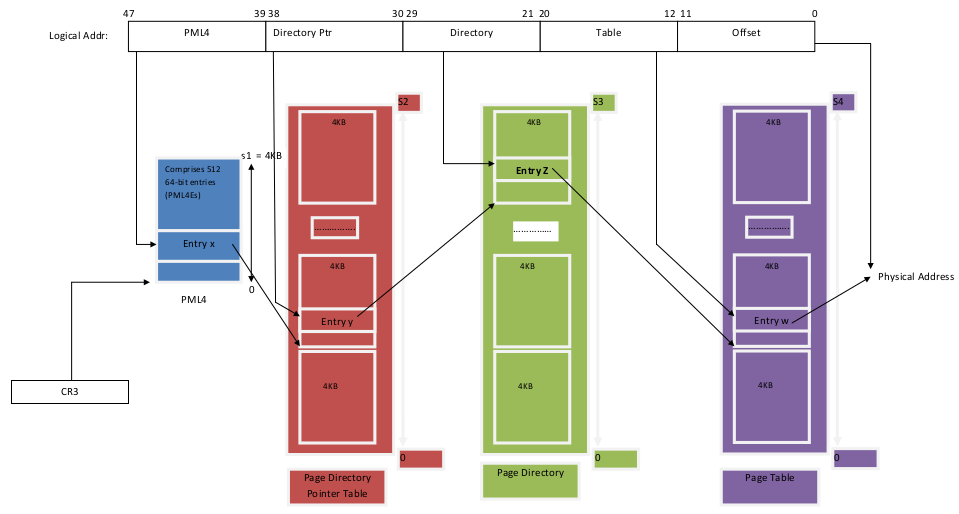}
\caption{Paging structure and translation.}
\label{fig:paging-structure-1}
\end{figure}

\begin{figure}
\includegraphics[scale=0.6]{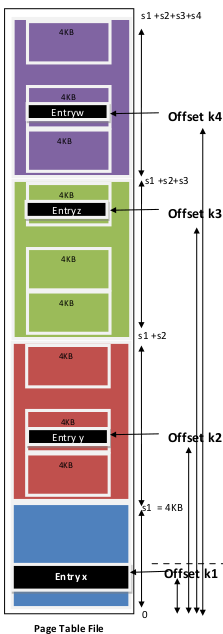}
\caption{Layout of the paging structure in memory.}
\label{fig:paging-structure-2}
\end{figure}
