# Supplementary material for: Verification of a Generative Separation Kernel
Source: arXiv:2001.10328 source file (2020-05-14)
Supplement: Supplementary file 2 [file appendix-interrupt-handling.tex]

\section{Event Handling} 
\label{app:appendix-interrupt-handling}

\begin{center}
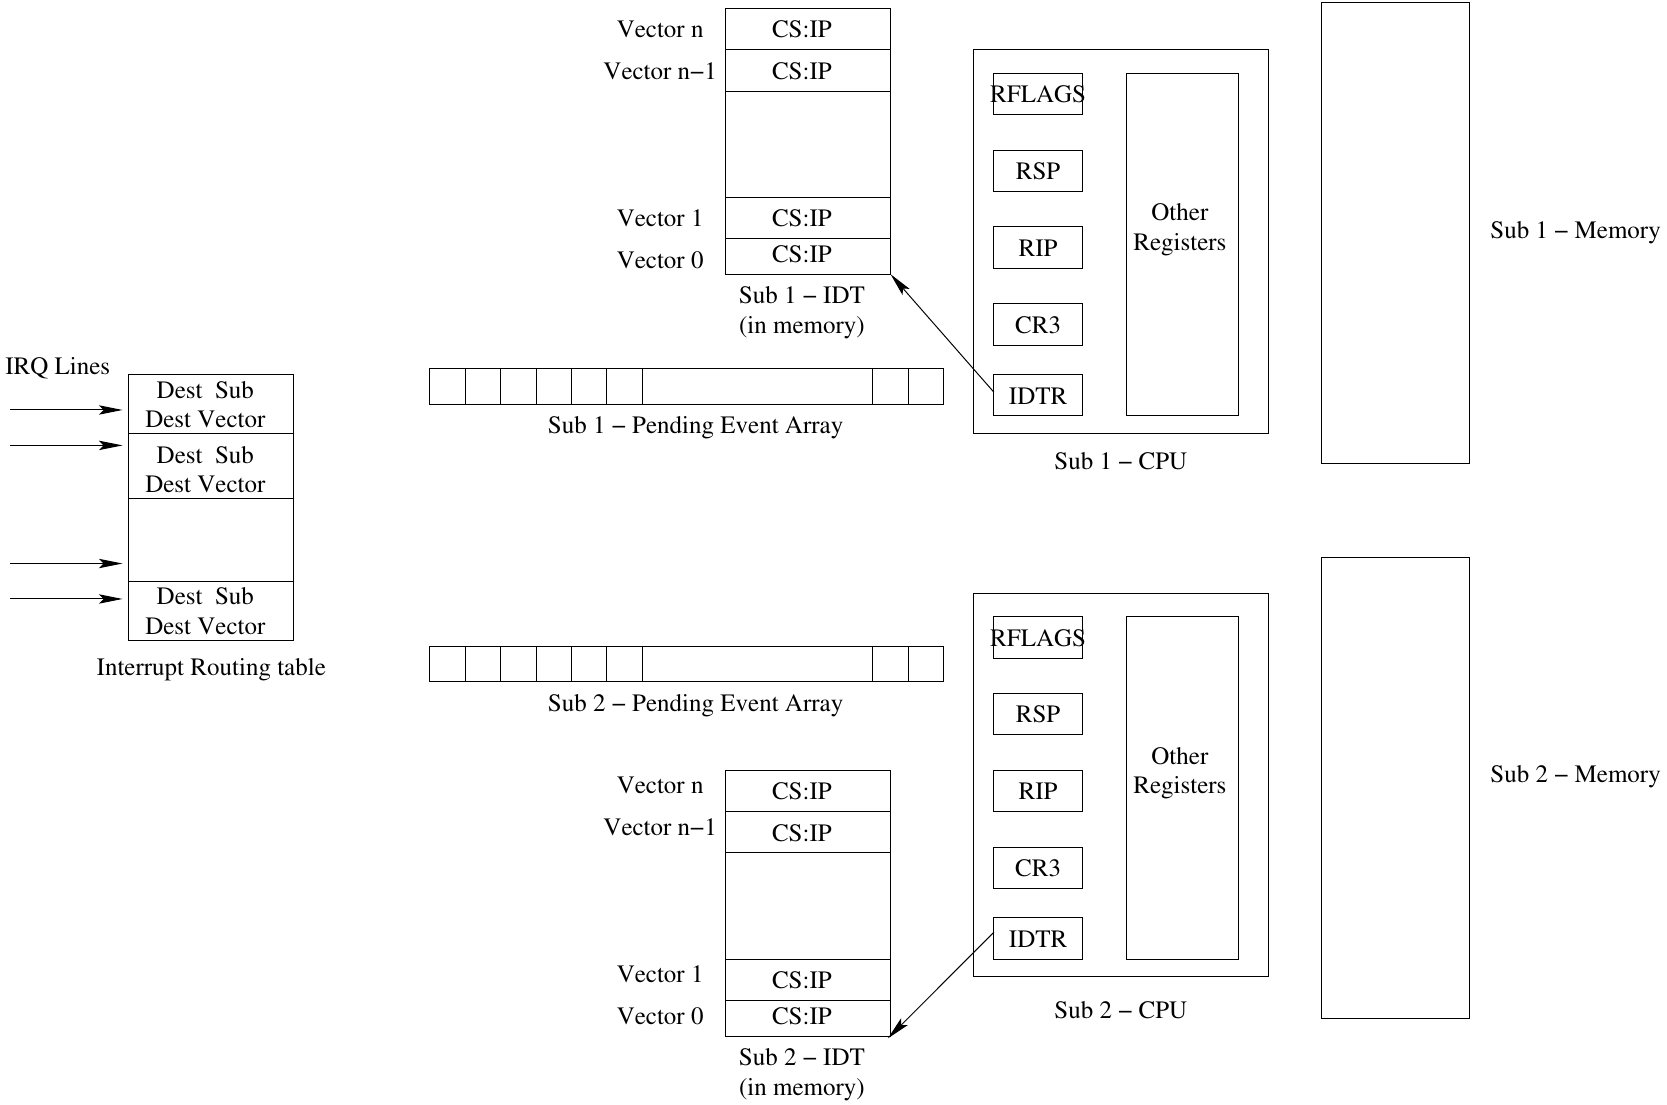
\end{center}

\begin{center}
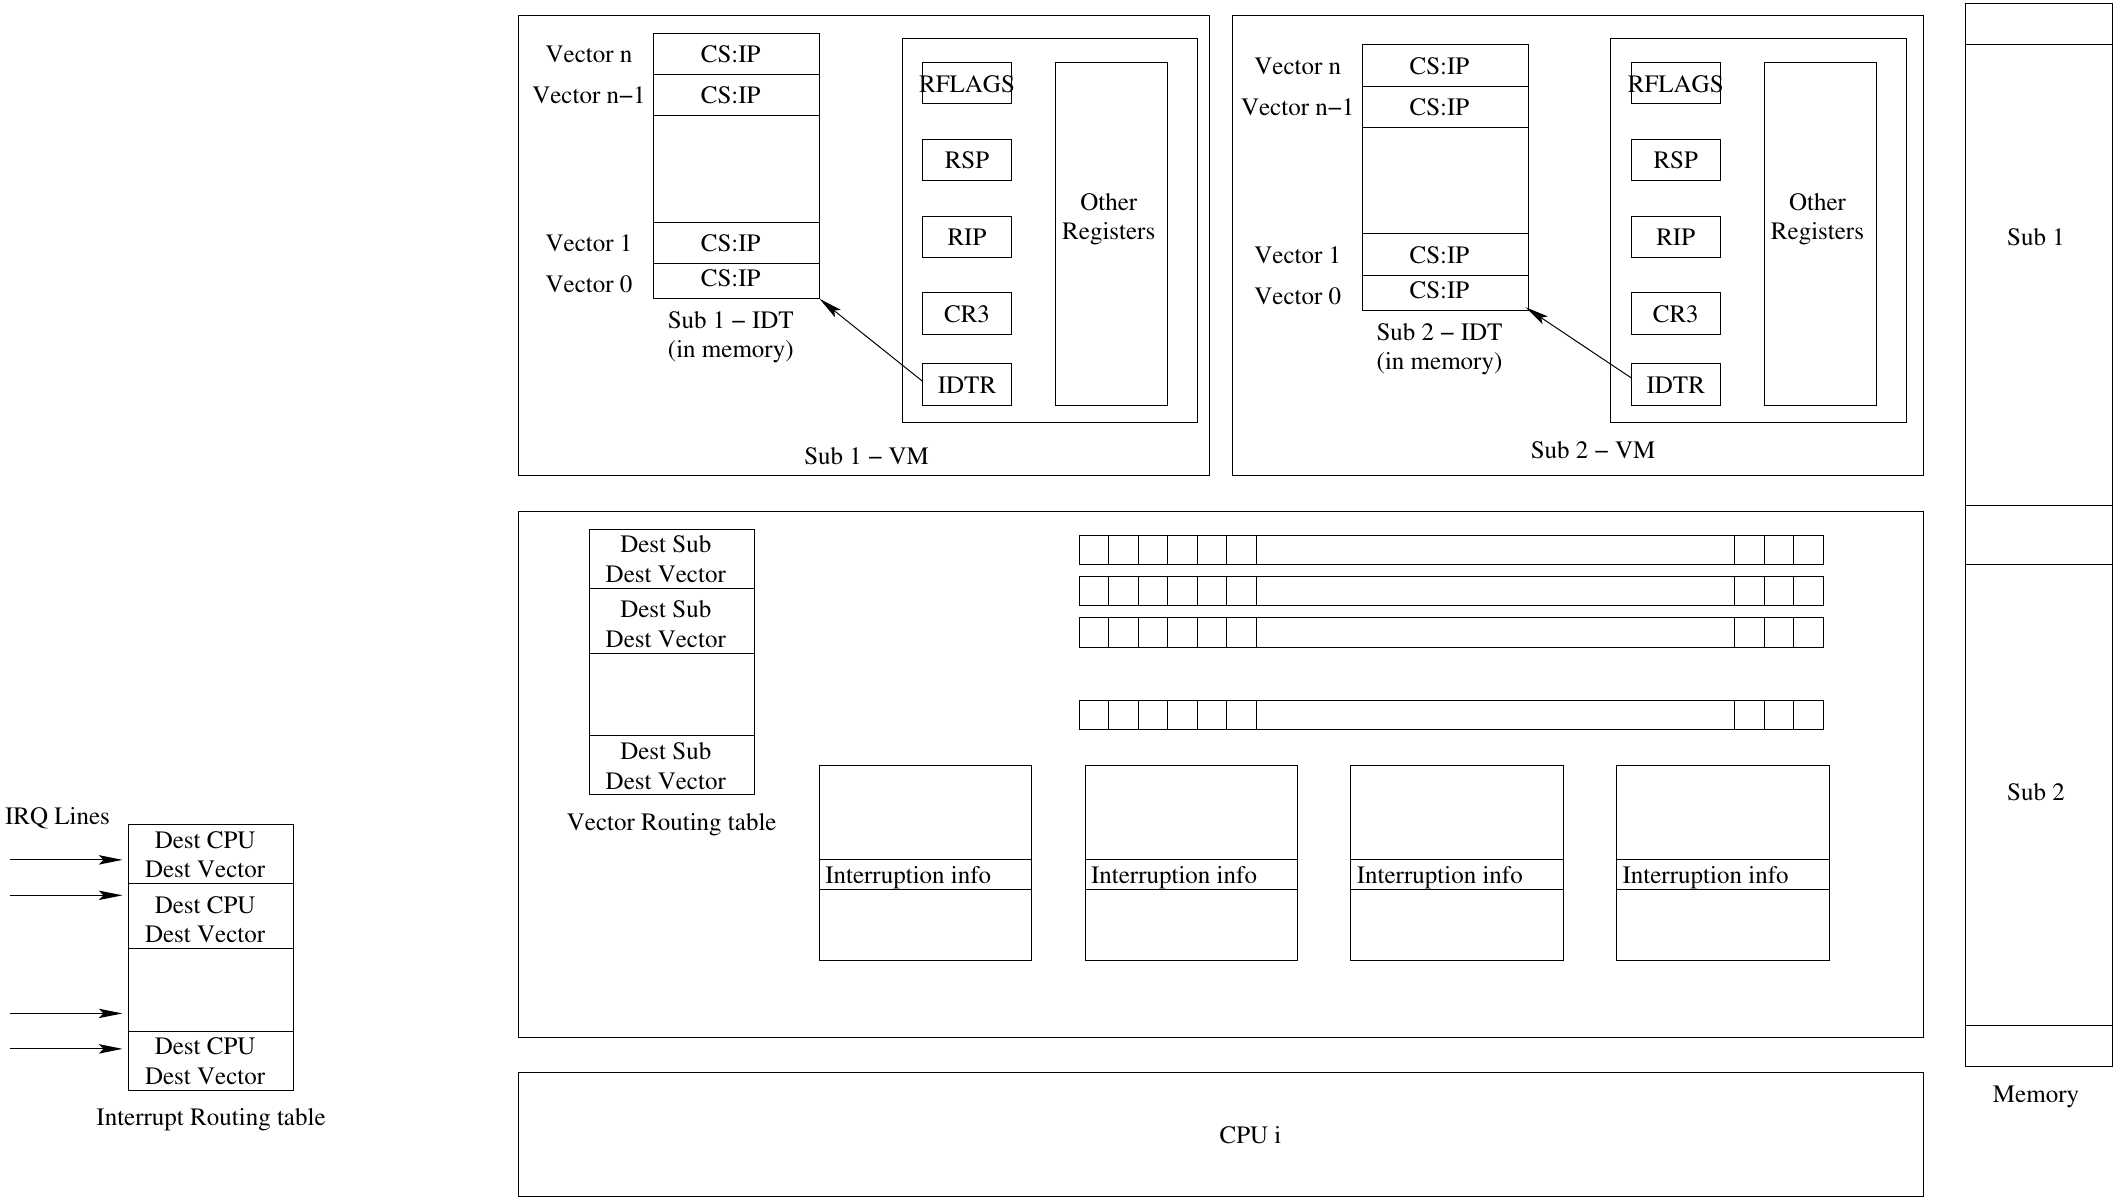
\end{center}
